# Supplementary material for: MoCHA: Denoising Caption Supervision for Motion-Text Retrieval
Source: arXiv:2603.23684 source file (2026-04-07)
Supplement: Supplementary file 1 [file appendices.tex]

\documentclass[runningheads]{llncs}

% ECCV 2026 formatting
\usepackage[review,year=2026,ID=*****]{eccv}

% Common abbreviations
\usepackage{eccvabbrv}

% Additional packages
\usepackage{graphicx}
\usepackage{booktabs}
\usepackage{multirow}
\usepackage{xcolor}
\usepackage{colortbl}
\usepackage{enumitem}
\usepackage{subcaption}
\usepackage{comment}
\usepackage{arydshln}

% Accessibility
\usepackage[accsupp]{axessibility}

% Hyperref (review version with pagebackref)
\usepackage[pagebackref,breaklinks,colorlinks,citecolor=eccvblue]{hyperref}

% Custom colors
\definecolor{darkgreen}{rgb}{0.0, 0.5, 0.0}
\definecolor{lightgray}{gray}{0.9}
\definecolor{bestcell}{rgb}{0.9, 0.95, 1.0}

% Custom commands

% Title
\title{Text Canonicalization for Cross-Dataset\\Motion-Text Retrieval\\[6pt]\Large Supplementary Material}
\titlerunning{Text Canonicalization for Motion-Text Retrieval -- Appendices}

% Authors (anonymized for review)
\author{Anonymous ECCV 2026 Submission}
\authorrunning{Anonymous}
\institute{Paper ID *****}

\begin{document}

\maketitle

\input{appendices_body}

%==============================================================================
% References (for standalone compilation)
%==============================================================================

\bibliographystyle{splncs04}

\end{document}
